# Supplementary material for: Monocular Per-Object Distance Estimation with Masked Object Modeling
Source: arXiv:2401.03191 source file (2025-02-04)
Supplement: Supplementary file 1 [file fig_qualitatives_supp.tex]

\onecolumn
\section{Bird's-eye-view qualitatives}
In the following, we show some qualitative results showcasing the effectiveness of \liftername \mom in estimating distances across KITTI, NuScenes, and MOTSynth datasets. These qualitative studies show our model's efficacy at estimating distances in scenarios where even human responses fall short of approximation.
\begin{figure*}[h]
    % kitti
    \centering
    \includegraphics[width=\textwidth]{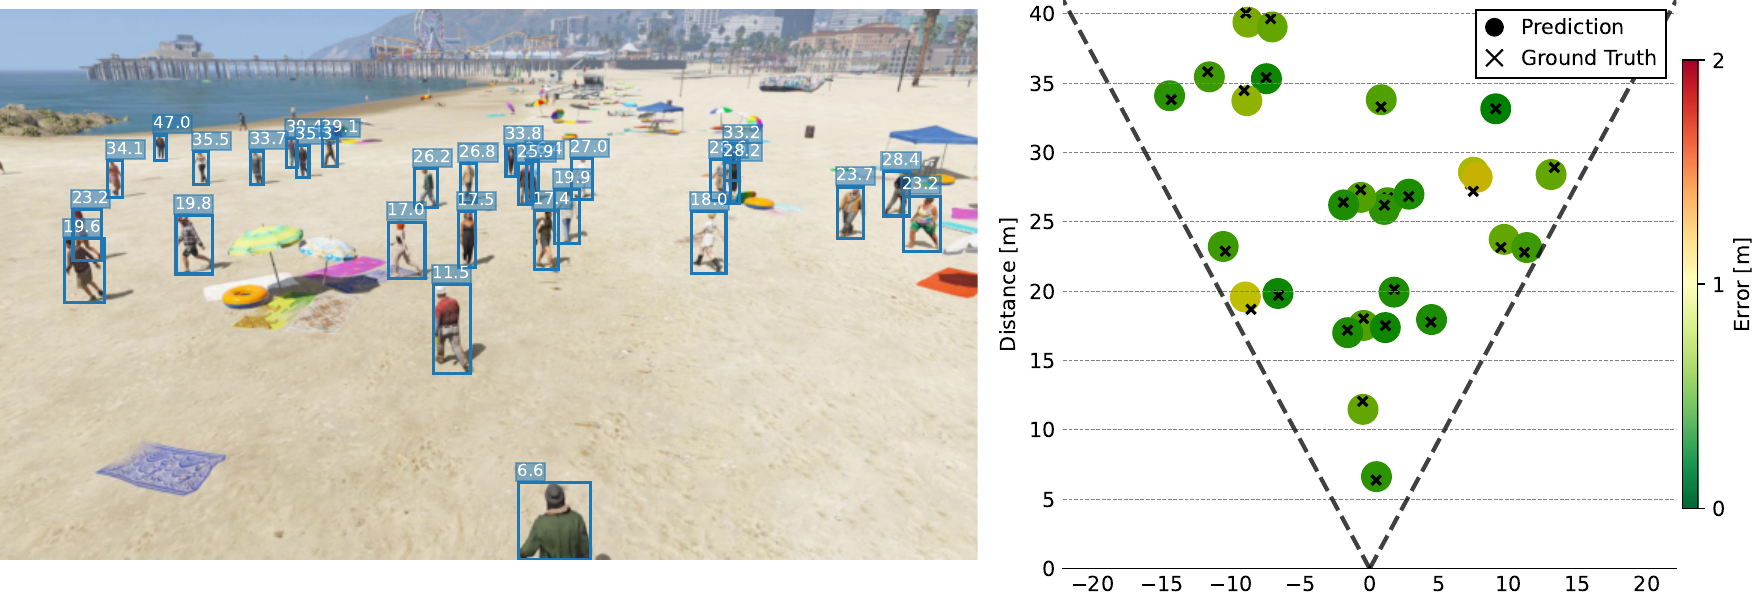}
    \includegraphics[width=\textwidth]{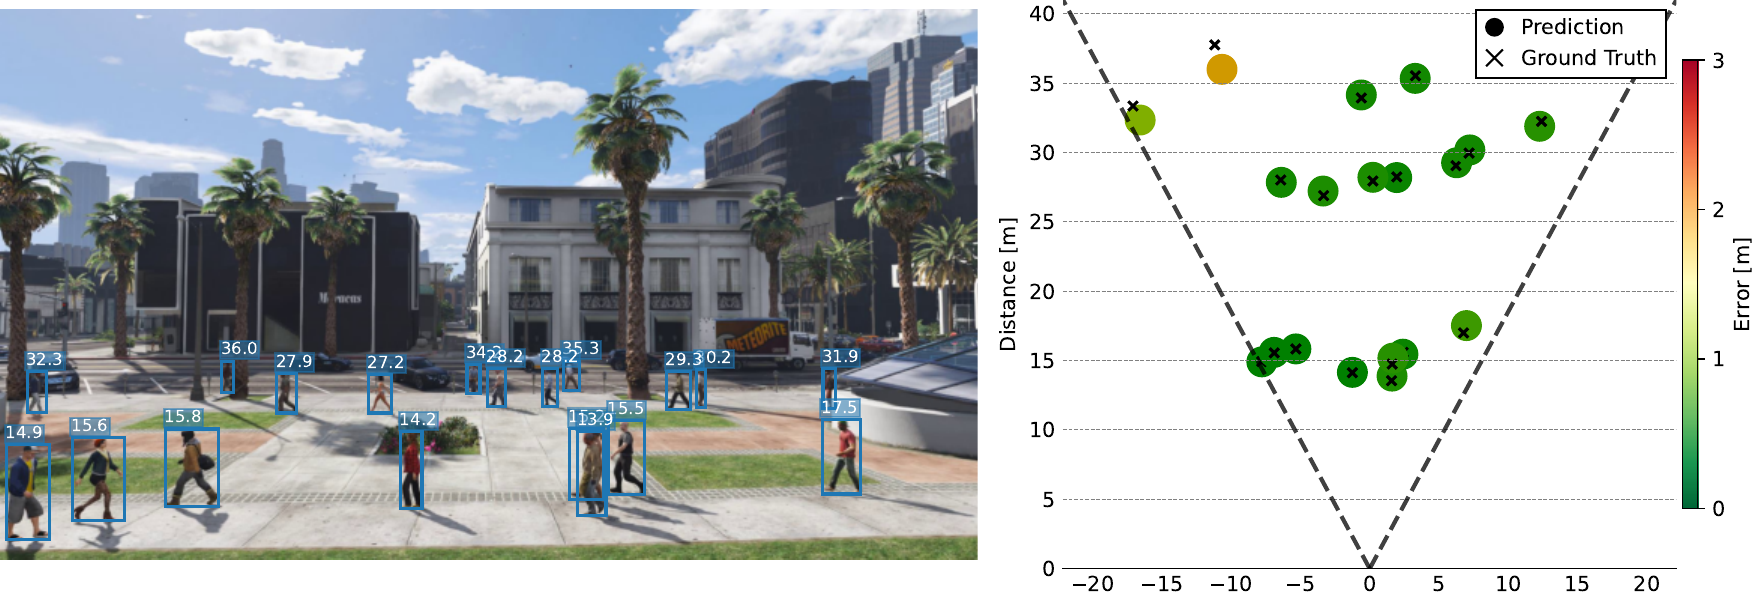}
\end{figure*}

\begin{figure*}[h]
    % nuscenes
    \centering
    \includegraphics[width=\textwidth]{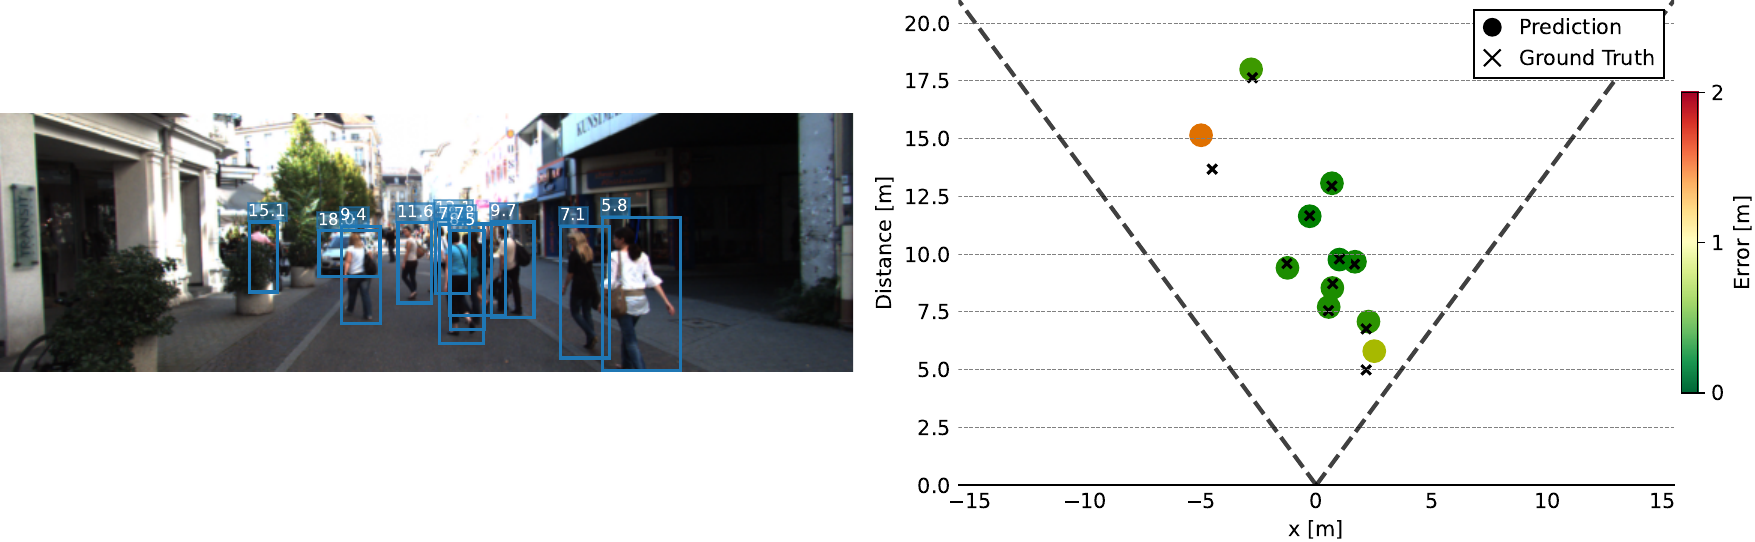}
    \includegraphics[width=\textwidth]{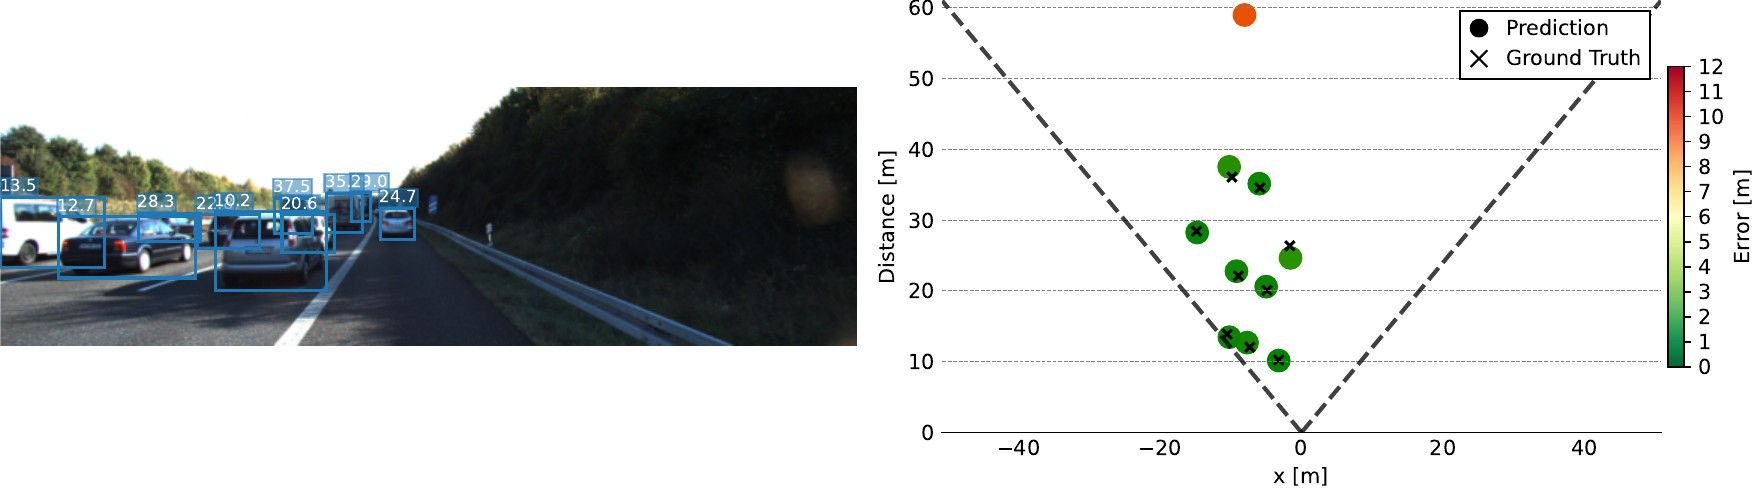}
\end{figure*}

\begin{figure*}[h]
    % motsynth
    \centering
    \includegraphics[width=\textwidth]{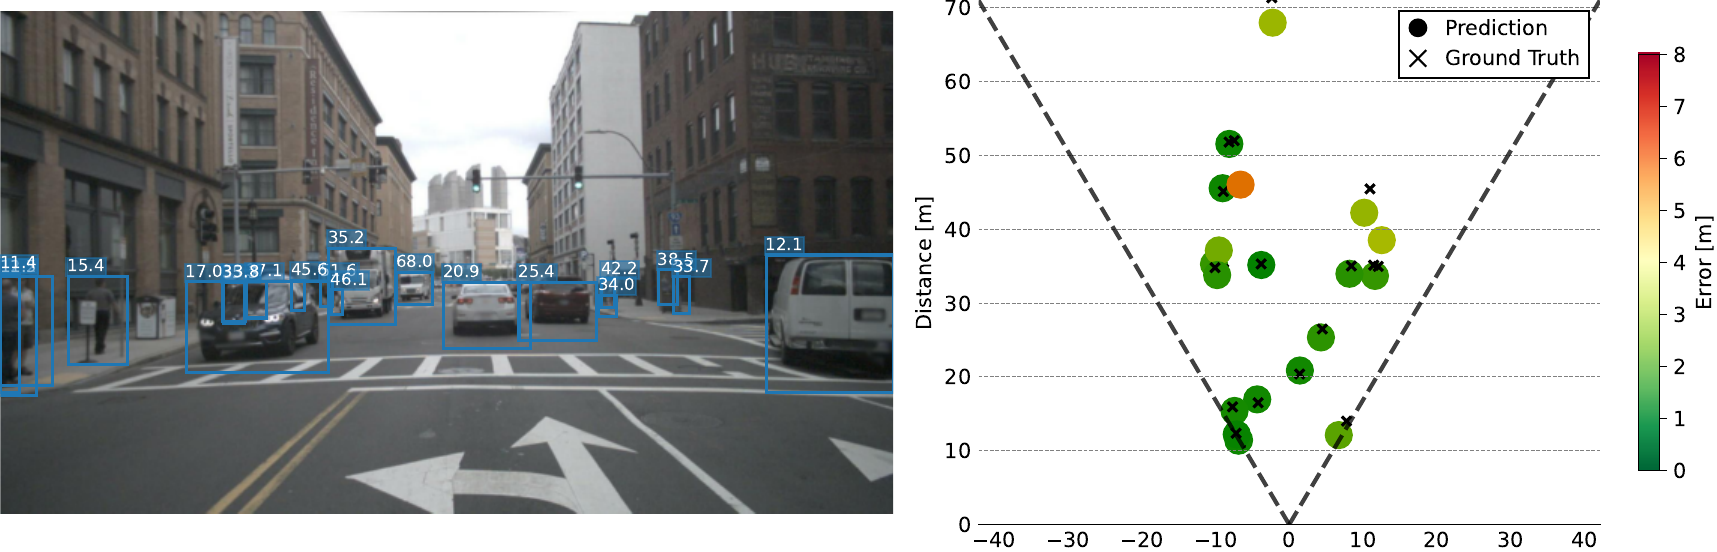}
    \includegraphics[width=\textwidth]{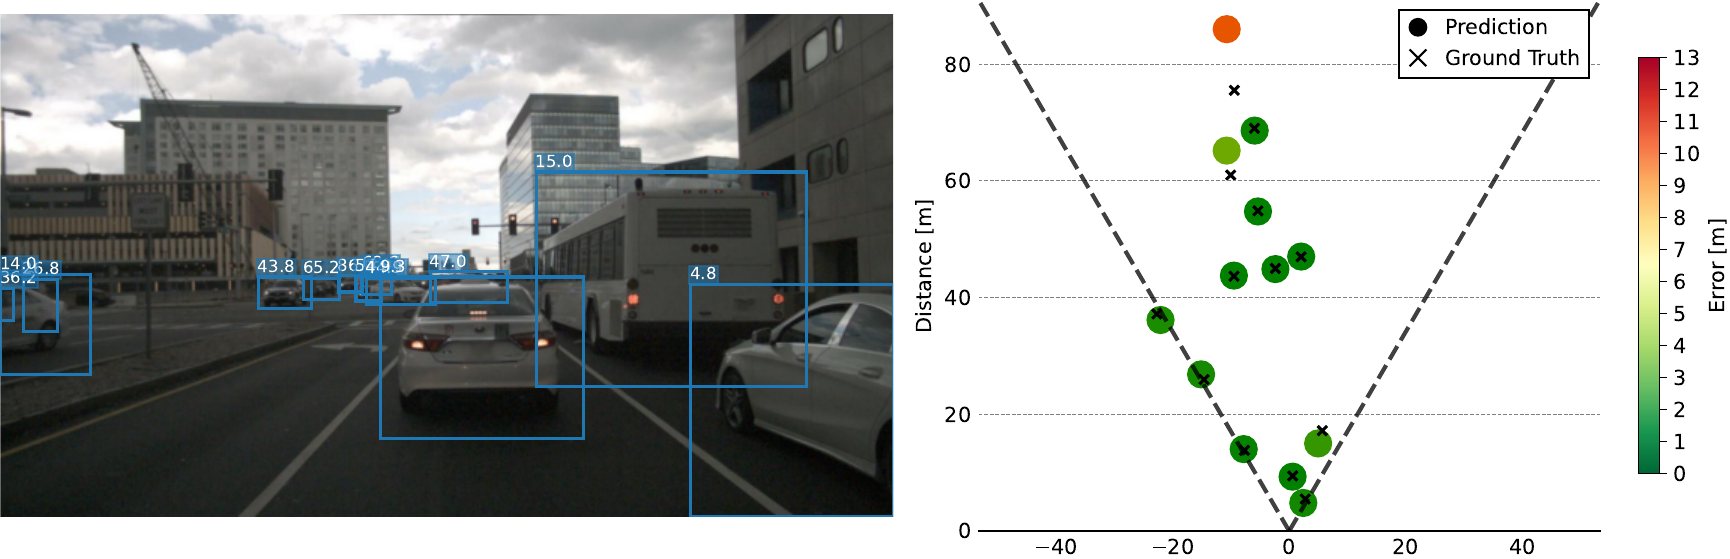}
\end{figure*}
