# Supplementary material for: Monocular Per-Object Distance Estimation with Masked Object Modeling
Source: arXiv:2401.03191 source file (2025-02-04)
Supplement: Supplementary file 2 [file fig_recon_supp.tex]

\begin{figure*}[tp]
    \centering
    \includegraphics[width=\textwidth,trim={0 4.6cm 0 0},clip]{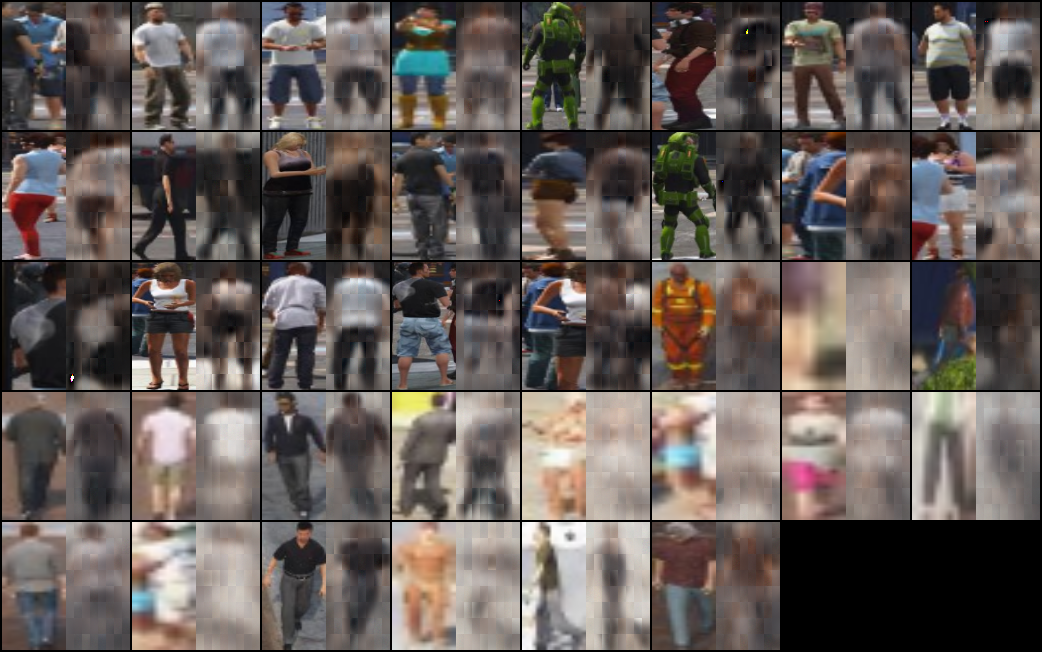}
    \caption{Qualitative examples of the reconstructions on MOTSynth. MoM tends to remove aesthetic details, such as colors, costumes and decorations, while keeping the shape of people.}
    \label{fig:art-mot}
\end{figure*}
